# Supplementary material for: Uni-FedRec: A Unified Privacy-Preserving News Recommendation Framework for Model Training and Online Serving
Source: arXiv:2109.05236 source file (2021-09-11)
Supplement: Supplementary file 1 [file Supplement.tex]

\section*{Supplementary Materials}

\subsection*{Experimental Environment}

In this section, we introduce the computer environment for performing experiments in our paper.
Experiments are conducted on a Linux server whose operating system is Ubuntu 16.04.6.
There are 7 Nvidia GeForce GTX 1080 Ti GPUs in the server, whose memory is 12 GB.
The server contains 32 Intel Xeon E5-2620 CPUs and 128-GB memory.
Besides, our deep models are implemented to run on a single GPU via the Keras framework.

\subsection*{Dataset Description}
Two datasets are used for experiments in our paper.
The first dataset is \textit{MIND}\footnote{https://msnews.github.io/index.html}, a large-scale public news recommendation dataset.
This dataset contains user logs collected from Microsoft News from October 12 to November 22 (6 weeks).
It contains 1,000,000 users, 161,013 news, 15,777,377 impressions, and 24,155,470 clicks in total.
User logs in the first 4 weeks are used to construct users' historical clicked news, user logs in the first 5 days of the 5-th week are used to construct training dataset, user logs in the last two days of the 5-th week are used to construct validation dataset, and user logs in the last week are used to construct test dataset.
Besides, the label of the test dataset of \textit{MIND} are not released and we can only obtain the ranking performance of models on given test impressions by submitting results to an official leaderboard.
We cannot evaluate the recall performance and overall recommendation performance of different methods on the test set.
Thus, we conduct experiments on the validation dataset due to the fact that click labels in the validation dataset are released publicly.

The second one is \textit{NewsFeeds}, which is constructed by logs of 20,000 users in a news feeds platform during two weeks (Mar. 18 to Apri. 1, 2020).
User logs in the first week are used to construct user historical behaviors, logs in the last two days are used for evaluation, and other logs are used for model training and validation.
It is composed of 120,219 news, 48,923 impressions, and 112,927 clicks.
We show more detailed information on \textit{MIND} and \textit{NewsFeeds} datasets in Table~\ref{table.deatiled.stat}.

\begin{table}[]
\centering
\resizebox{0.4\textwidth}{!}{\begin{tabular}{lcc}
\Xhline{1pt}
                              & \textit{MIND}    & \textit{NewsFeeds}     \\ \hline
\# News                        & 161,013  & 120,219 \\
\# Users                       & 1,000,000  & 20,000    \\
\# Impressions                 & 15,777,377 & 48,923   \\
\# Clicks                      & 24,155,470 & 112,927   \\
Avg. \# words in news title    & 11.78   & 11.90     \\
\Xhline{1pt}
\end{tabular}
}
\caption{Statistics of the \textit{MIND} and \textit{NewsFeeds} datasets.}
\label{table.deatiled.stat}
\end{table}

\subsection{Ranking Model}
\label{sec.sup.rank}
In this section, we introduce the settings of ranking models used in our experiments.

The first one is \textit{FedNewsRec}.
It stacks a word embedding layer, a CNN network, a multi-head self-attention network, and an attention pooling network to learn news embedding from news titles.
It learns short-term user interest embeddings from users' recent clicked news via a GRU network and learns long-term user interest embeddings from users' clicked news via a multi-head self-attention network.
It further builds a unified user interest embedding by aggregating short- and long-term user interest representation via an attention network.
In our experiments, for the news modeling method, the CNN network is set to have 256 filters, the multi-head self-attention network is set to have 16 attention head and output vectors of each head are 16-dimensional, i.e., ($16\times 16$), and the attention network is a two-layer dense network with 128-dimensional vectors.
For user modeling, the multi-head self-attention network is set to $16\times16$, the hidden states of the GRU network are 256-dimensional, and the attention network is also a two-layer dense network with 128-dimensional vectors.

The second one is \textit{NRMS}.
It stacks a word embedding layer, a multi-head self-attention network, and an attention network to learn news embeddings from news titles.
It stacks a multi-head self-attention network and an attention pooling network to learn user interest embeddings from representations of user's clicked news.
In our experiments, for news modeling, the multi-head self-attention network is set to $16\times 16$, and the attention network is a two-layer dense network with 128-dimensional hidden vectors.
For user modeling, the multi-head self-attention network is set to $16\times16$, and the attention network is a two-layer dense network with 128-dimensional hidden vectors.

The third one is \textit{LSTUR}.
It first stacks the word embedding layer, a CNN network, and an attention pooling network to learn title embeddings from news titles.
It further builds topic embeddings from news topics via a topic embedding layer and further combines topic and title embeddings via a dense network to learn unified representations for news.
Besides, it employs a GRU network to learn short-term user interest embeddings from the sequence of user's clicked news and employs a user ID embedding to learn long-term user interest embeddings.
It further builds a unified user interest embedding by combining short- and long-term user interest embeddings via a dense network.
In our experiments, for news modeling, the CNN network is set to contain 256 filters, the attention network is a two-layer dense network with 128-dimensional hidden vectors, the topic embedding layer is initialized by 100-dimensional randomly-generated vectors, and the dense network is set to output 256-dimensional output vectors.
For user modeling, the hidden states of the GRU network are 256-dimensional, the ID embeddings are 256-dimensional and randomly initialized, and the dense network is set to output 256-dimensional output vectors.

The forth one is \textit{NAML}.
Following Wu et al.~\cite{wu2020mind}, we only used news titles in \textit{NAML}.
Specifically, we stack a word embedding layer, a CNN network, and an attention network to learn news embeddings from news titles.
Besides, \textit{NAML} employ an attention network to learn user interest embedding from embeddings of user's clicked news.
In our experiments, the CNN network contains 256 filters, and the two attention networks are dense networks with 128-dimensional vectors.

Besides, we used 300-dimensional glove embeddings to initialize word embedding layers.

\subsection*{Data Preprocessing}

We compare different models based on the same data preprocessing method for fair comparisons.
For the preprocessing of news, we use the word tokenizer of an open-source library, i.e., NLTK\footnote{https://www.nltk.org/} to split words of news titles.
We only use the first 30 words in news titles.
To model user interests, we only use 50 recent clicked news of each user.

\subsection*{Hyperparameter Settings}
In this section, we introduce all hyperparameter settings of our method.
In our experiments, representations of both news and user are $256$ dimensional.
More specifically, in our recall model, the self-attention network contains $16$ attention heads with $16$-dimensional output vectors.
The clustering distance $d_c$ is set to 2.
The cluster-wise attention network is implemented by a two-layer dense network with 128-dimensional vectors.
The number ($B$) of \textit{CGIE} is set to 30 and the dimensions of these embeddings are 256.
The intensity $\lambda_I$ of the Laplace noise $n_I$ is set to 1.2.
Embeddings generated by the news model and user model in these ranking methods are $256$-dimensional.
Detailed settings of these ranking models are in Section~\ref{sec.sup.rank}.
For each updating step of model training, we sample $r=2\%$ clients from all clients.
The gradient clipping value is set to $0.1$ and intensity $\lambda_g$ of noise $n_g$ is $0.01$.
The learning rate $\omega$ is set to 0.05. 
Besides, we also apply dropout technique~\cite{srivastava2014dropout} with $0.2$ dropout probability to each layer for more effective model training.

\subsection*{Performance Evaluation}

In this section, we introduce evaluation metrics, i.e., R@K AUC, MRR, nDCG@5, and nDCG@10 used in this paper.
R@K is a widely used metric to measure recall accuracy:
\begin{equation}
    R@K = \sum_{u\in \mathcal{U}_a} \frac{|\mathcal{C}_u \bigcap \mathcal{R}_K |}{|\mathcal{C}_u|},
\end{equation}
where $\mathcal{U}_a$ denotes the set of all users in the dataset, $\mathcal{C}_u$ is the set of clicked news of the user $u$, and $\mathcal{R}_K$ is the set of top K recalled news.

AUC is a widely used ranking metric:
\begin{equation}
    AUC = \frac{1}{|\mathcal{T}_p||\mathcal{T}_n|}\sum_{n_p\in \mathcal{T}_p}\sum_{n_n\in \mathcal{T}_n} \mathcal{I}(\hat{y}^p>\hat{y}^n),
\end{equation}
where $\mathcal{T}_p$ is the set of positive samples in the impression, $\mathcal{T}_n$ is the set of negative samples in the impression, $\hat{y}^p$ is the matching score of the positive sample, $\hat{y}^n$ is the matching score of the negative sample, and $\mathcal{I}(\cdot)$ is a indicator function.

MRR is calculated as follow:
\begin{equation}
    MRR=\frac{1}{ |\mathcal{T}_p| }\sum_{ p_i \in \mathcal{T}_p } \frac{1}{r(p_i)},
\end{equation}
where $p_i$ is the $i-$ th positive sample in set $\mathcal{T}_p$, and $r(p)$ denotes the ranking position of $p$.

Besides, nDCG@K is calculated as follow:
\begin{equation}
    nDCG@K=\frac{\sum_{i=1}^{K}(2^{y_i}-1)/\log_2(1+i)}{ \sum_{i=1}^{ |\mathcal{T}_p| }1/\log_2(1+i)},
\end{equation}
where $y_i$ is the label of the $i$-th sample ranked by the algorithm.
Codes of these ranking metrics can be found in code file ``UniFedRec.ipynb'' (the penultimate cell).

\subsection*{Performance on Validation Sets}
We manually tuned hyper-parameters of different methods based on their results on the validation set.
Table~\ref{table.valid} shows the validation results.

\begin{table}[]
\centering
\resizebox{0.48\textwidth}{!}{
\begin{tabular}{c|cccc}
\Xhline{1pt}
          & R@100 & R@200 & R@300 & R@400 \\ \hline
AVG     & 2.41 & 3.41 & 3.99 & 4.88     \\
ATT     & 2.67 & 3.73 & 4.05 & 4.60   \\
GRU     & 3.74 & 5.85 & 7.53 & 8.90  \\
SelfAtt & 4.06 & 6.07 & 7.78 & 9.13   \\
PinnerSage & 1.97 & 3.26 & 4.26 & 5.03  \\
Octopus    & 1.95 & 3.27 & 4.22 & 5.00\\ \hline
UniFedRec  & 4.92 &7.31 & 9.02 &10.41\\ \Xhline{1pt}
\end{tabular}
}
\caption{Validation results of different methods.}
\label{table.valid}
\end{table}
%{100: 2.4125874125874125, 200: 3.4115884115884114, 300: 3.994338994338994, 400: 4.88011988011988, 500: 5.362970362970363}
%{100: 2.667997338656021, 200: 3.7325349301397206, 300: 4.048569527611444, 400: 4.597471723220226, 500: 5.09647371922821}
%{100: 3.743526089631547, 200: 5.85499200956508, 300: 7.537761813303543, 400: 8.902967712850105, 500: 10.122988304180877}
%{100: 4.0633940907489015, 200: 6.072677895368924, 300: 7.780594318969641, 400: 9.130728949426569, 500: 10.412210459620976}
%{100: 1.9655578766939847, 200: 3.2665857244034973, 300: 4.25763743817737, 400: 5.032371182539912, 500: 5.5361251775762454}
%{100: 1.9544183319049124, 200: 3.271610507164659, 300: 4.222266494922004, 400: 5.004409920734519, 500: 5.515815988266256}
%{100: 4.924709498718395, 200: 7.313732071465971, 300: 9.015529212021788, 400: 10.409451868027118, 500: 11.766736602741695}

\subsection*{Efficiency of Our Model}

The ranking model of \textit{UniFedRec} contains 1.01 MB parameters.
Besides, it takes about 200 rounds to train the recall model until model convergence the on \textit{MIND} dataset.
It takes about 50 rounds to train the recall model until model convergence the on \textit{NewsFeeds} dataset.

% \subsection*{Influence of Clustering Distance}

% \begin{figure}
%     \centering
%     \resizebox{0.4\textwidth}{!}{
%     \includegraphics{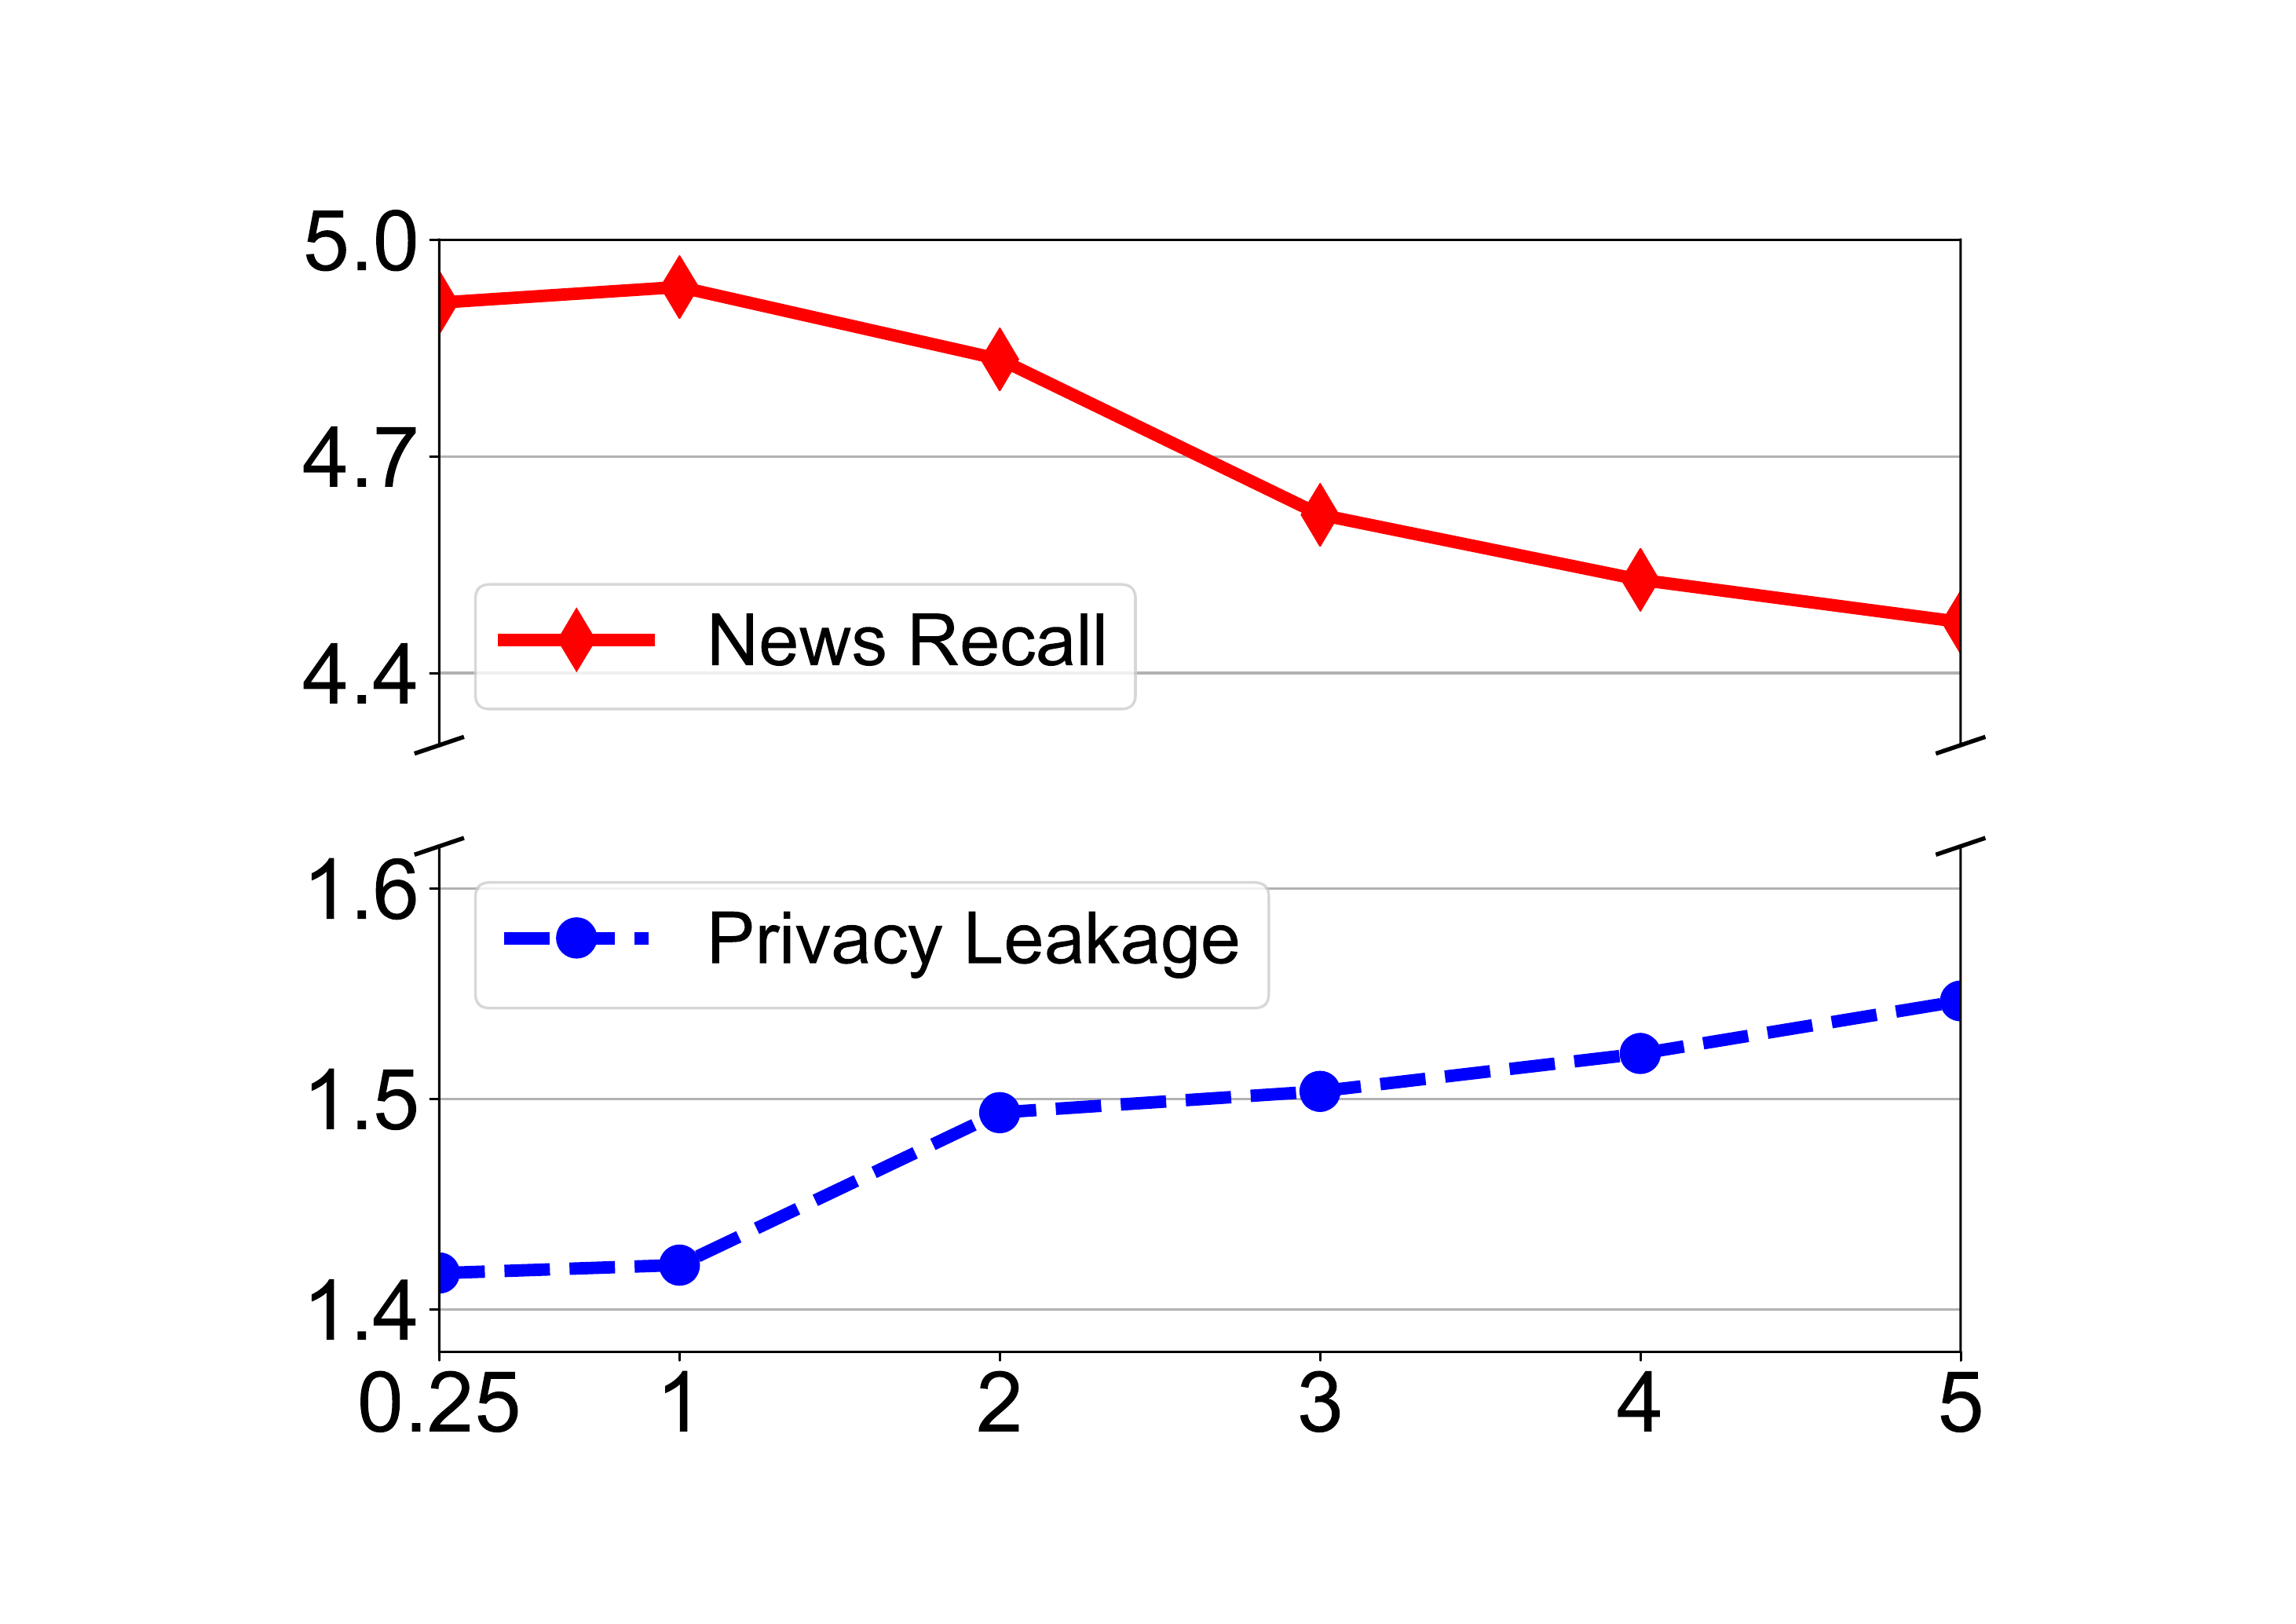}
%     }
%     \caption{Influence of clustering distance on \textit{UniFedRec}.}
%     \label{fig.distance}
% \end{figure}

% As shown in Fig.~\ref{fig.distance}, we shown influence of clustering distance $\textit{d}_c$ on \textit{UniFedRec}.
% We can find that with the increase of $d_c$, recall accuracy first increases.
% This is because when $d_c$ is too small, we clustering user's clicked news into too many interest clusters, which may bring much noise and hurt recall accuracy.
% Second, when $d_c$ becomes large enough, recall accuracy begins to decline.
% This is because when $d_c$ becomes too large, much fewer interest clusters will be formed and their representations is sufficient to comprehensively model diverse user interests. 
% Third, we can find with the increase of $d_c$, the privacy protection ability of \textit{UniFedRec} declines.
% This may be because applying our proposed interest decomposer-aggregator framework to interest representations with more channels can more effectively protect user privacy.
% Thus, a moderate value of $d_c$, e.g., 1, is suitable for \textit{UniFedRec}.
